# Supplementary material for: Active Learning with Context Sampling and One-vs-Rest Entropy for Semantic Segmentation
Source: arXiv:2412.06470 source file (2025-03-17)
Supplement: Supplementary file 1 [file 7_supplementary_materials.tex]

% % WACV 2025 Paper Template
% % based on the WACV 2024 template, which is
% % based on the CVPR 2023 template (https://media.icml.cc/Conferences/CVPR2023/cvpr2023-author_kit-v1_1-1.zip) with 2-track changes from the WACV 2023 template (https://github.com/wacv-pcs/WACV-2023-Author-Kit)
% % based on the CVPR template provided by Ming-Ming Cheng (https://github.com/MCG-NKU/CVPR_Template)
% % modified and extended by Stefan Roth (stefan.roth@NOSPAMtu-darmstadt.de)

% \documentclass[10pt,twocolumn,letterpaper]{article}

% %%%%%%%%% PAPER TYPE  - PLEASE UPDATE FOR FINAL VERSION
% %\usepackage[review,algorithms]{wacv}      % To produce the REVIEW version for the algorithms track
% %\usepackage[review,applications]{wacv}      % To produce the REVIEW version for the applications track
% \usepackage{wacv}              % To produce the CAMERA-READY version
% %\usepackage[pagenumbers]{wacv} % To force page numbers, e.g. for an arXiv version

% % Include other packages here, before hyperref.
% \usepackage{graphicx}
% \usepackage{algorithm}
% \usepackage{algpseudocode}
% \usepackage{amsmath}
% \usepackage{amssymb}
% \usepackage{booktabs}
% \usepackage{diagbox}
% \usepackage{bm}
% \usepackage{enumitem}

% % It is strongly recommended to use hyperref, especially for the review version.
% % hyperref with option pagebackref eases the reviewers' job.
% % Please disable hyperref *only* if you encounter grave issues, e.g. with the
% % file validation for the camera-ready version.
% %
% % If you comment hyperref and then uncomment it, you should delete
% % ReviewTempalte.aux before re-running LaTeX.
% % (Or just hit 'q' on the first LaTeX run, let it finish, and you
% %  should be clear).
% \usepackage[pagebackref,breaklinks,colorlinks]{hyperref}


% % Support for easy cross-referencing
% \usepackage[capitalize]{cleveref}
% \crefname{section}{Sec.}{Secs.}
% \Crefname{section}{Section}{Sections}
% \Crefname{table}{Table}{Tables}
% \crefname{table}{Tab.}{Tabs.}


% %%%%%%%%% PAPER ID  - PLEASE UPDATE
% \def\wacvPaperID{623} % *** Enter the WACV Paper ID here
% \def\confName{WACV}
% \def\confYear{2025}


% \begin{document}

% \input{def}
% %%%%%%%%% TITLE - PLEASE UPDATE
% \title{Supplementary Materials: Active Learning with Context Sampling and One-vs-Rest Entropy for Semantic Segmentation}

% \author{
%     Fei Wu$^{1}$, Pablo Marquez-Neila$^{1}$, Hedyeh Rafii-Tari$^{2}$, Raphael Sznitman$^{1}$\\
%     $^{1}$University of Bern \\ 
%     $^{2}$Johnson \& Johnson \\
%     {\tt\small \{fei.wu,pablo.marquez,raphael.sznitman\}@unibe.ch}\\
%     {\tt\small hrafiita@its.jnj.com}
% }
% \maketitle
% % \input{def}
% % \input{sec/0_abstract}
% % \input{sec/1_introduction}
% % \input{sec/2_related_works}
% % \input{sec/3_method}
% % \input{sec/4_experiments}
% % \input{sec/5_results}
% % \input{sec/6_conclusion}

% %%%%%%%%% REFERENCES
% % {\small
% % \bibliographystyle{ieee_fullname}
% % \bibliography{main}
% % }

% \section{A simple experiment to test the efficiency of context sampling.}

% While we argue it is important to create context around objects we want to segment to further improve the segmentation accuracy, we wanted to confirm this behavior with a simple experiment. After splitting images into several superpixel patches, each superpixel is assigned the most prominent pixel label that it contains. We compare two sampling strategies: The first one selects superpixels from foreground classes with high probability and the second one acts the same as the first one but also selects background superpixels located around foreground superpixels (context) with high probability. The results displayed in Fig.~\ref{fig: random weight} confirm our hypothesis that labeling the context around objects we want to segment improves the segmentation accuracy. Indeed the Active Leaning (AL) curve of \emph{foregrounds + context} is always above the one of \emph{foregrounds}.

% \begin{figure}[t]
%     \includegraphics[width=\linewidth]{figures/intuitive_ResNet50_randomWeighted.pdf}
%    \caption{Comparison between a strategy that mainly samples foreground superpixels against a strategy that does the same but additionally samples superpixels in the immediate proximity of foreground superpixels as well. Values are averaged over 10 training-validation splits. Error bars indicate one standard deviation.}
% \label{fig: random weight}
% \end{figure}

% \section{OVR entropy and \OurSamp}
% In this section, we provide further details on \OurSamp~.
% \subsection{Class Balacing}
% We go back to the Sec. 3.5 of the main paper and explain more in detail how \OurSamp~balances the number of items per class using the OVR entropy. As mentioned in the main paper: "\emph{For high OVR entropy~$H_c$, the selected elements are the most uncertain for class~$c$. However, uncertain samples of class~$c$ do not guarantee that they are actually from that class, potentially resulting in a deviation from the predetermined~$\delta_c$. However, in practice, this discrepancy does not significantly impact class balance, as any deviation from~$\delta_c$ is compensated for in subsequent iterations.}"

% Such behavior is illustrated in Fig.~\ref{fig:toy_dataset} through the application of \OurSamp~on a toy dataset. The first batch selected for class 1 contains points from classes 2 and 3. However, batches selected for classes 2 and 3 contain points from class 1 as well, which compensated for the missing class-1 points in the first batch. Once all the points are selected, an oracle will provide the true label for all points no matter which class they were selected for.


% \begin{figure*}[t]
% \includegraphics[width=0.23\linewidth]{figures/toyDataset_OVR_class0.pdf}
% \includegraphics[width=0.23\linewidth]{figures/toyDataset_OVR_class1.pdf}
% \includegraphics[width=0.23\linewidth]{figures/toyDataset_OVR_class2.pdf}
% \includegraphics[width=0.23\linewidth]{figures/toyDataset_OVR_class3.pdf}
% \caption{Illustration of our sampling method \OurSamp~on a toy dataset. Starting with class 1, we calculate the OVR entropy of all samples for this class and select the samples with the highest OVR entropy. We repeat this process for the following classes iteratively. The number of samples to select per class depends on the number of labeled samples per class, the fewer labels we have for this class the more we select for it.}
% \label{fig:toy_dataset}
% \end{figure*}

% \subsection{Background class}
% \label{sec:background_class}

% Some datasets feature a background class that aggregates many different visual elements and exhibits high visual variability. For these datasets, balancing the background class with the other classes may result in insufficient coverage of its larger variability. We have observed a positive effect when oversampling the background class, which is achieved by simply enforcing~$n_b=0$ when computing class counts in Alg.~\ref{alg:compute_delta}, where $b$~is the index of the background class. This results in more selected superpixels~$\delta_b$ for the background class.

% %% compute delta algorithm
% \begin{algorithm}
% \caption{Required items per class}
% \Comment{{\footnotesize Solution to Eq. 3 in the main paper}}
% \label{alg:compute_delta}
% \begin{algorithmic}[1]
% \Require $\{n_c\}_{c=1}^C$ (current number of labeled items per class in $\A_t$), $Q$ (number of items to select for annotation)
% \Ensure $\{\delta_c\}_{c=1}^C$ (number of items to select per class)
% \Function{ItemsPerClass}{$\bm{n}$, $Q$}
% \State $\bm{\delta}\leftarrow \mathbf{0}$
% \While {$Q > 0$} 
%     \State $c \leftarrow {\arg\min}_c n_c + \delta_c$
%     \Statex \Comment{{\footnotesize Get the most underrepresented class~$c$}}
%     \State $\delta_c \leftarrow \delta_c + 1$
%     \Statex \Comment{{\footnotesize Increment the queried items for the class~$c$}}
%     \State $Q \leftarrow Q - 1$ \Comment{{\footnotesize Decrement the available budget}}
% \EndWhile

% \State \Return $\bm{\delta}$
% \EndFunction
% \end{algorithmic}
% \end{algorithm}

% \subsection{OREAL ablations}. We perform different ablations of our method to measure the contribution of each component to the final performance. Results of the ablation are shown in Table~\ref{tab: ablation} and Fig.~\ref{fig: ablation_AL_curves}. Our OVR entropy and the use of \MaxAgg have the largest effect on the final performance, while the oversampling of the background classes helps to improve the performance by a lesser but not negligible margin.
% \begin{description}[topsep=0pt, partopsep=0pt, leftmargin=*, labelindent=\parindent, itemindent=1em]
%     \item[\OurSamp~\MeanAgg.] We use the mean of pixel-wise OVR entropy scores instead of their maximum to compute superpixel OVR entropy.
%     \item[\OurSamp~Proba$\times$Entropy.] Substitute the OVR~entropy for an uncertainty measure obtained as the product of entropy times the predicted probability vector. The goal of this ablation is to compare the use of OVR entropy and the vanilla entropy \cite{entropy} when using class balance.
%     \item[\OurSamp~$\delta$.] We omit the special treatment of the background class (Sec.~\ref{sec:background_class}) for the datasets where it is applied (MONARCH, EndoVis, Pascal~VOC).\\
%     \RebuttalText{\item[\OurSamp~$95\%$.] Instead of using the max aggregation, we take the $95\%$ percentile pixel value to represent the superpixel.\\}
% \end{description}

% \begin{figure*}[t]
%     \includegraphics[width=0.5\linewidth]{figures/cityscapes_RN50_ablation.pdf}
%     \includegraphics[width=0.5\linewidth]{figures/pascal_VOC_RN50_ablation.pdf}
%     \medskip
%     \includegraphics[width=0.5\linewidth]{figures/auris_RN50_ablation.pdf}
%     \includegraphics[width=0.5\linewidth]{figures/intuitive_RN50_ablation.pdf}
%    \caption{Comparison of different ablation strategies.
%    Values are averaged over 3 training-validation splits for Cityscapes \cite{cityscapes}, Pascal VOC \cite{pascalVOC}, and 10 training-validation splits for EndoVis \cite{endovis}, MONARCH \cite{COWAL}. Error bars indicate one standard deviation.}
% \label{fig: ablation_AL_curves}
% \end{figure*}

% \begin{table*}
% \centering
% \resizebox{\textwidth}{!}{% Resize table to fit within the textwidth
% \begin{tabular}{c | c | c | c | c | c | c}
% Strategy & Cityscapes & Pascal VOC & MONARCH & EndoVis & Average & Avg /Cityscapes\\
% \hline
% OREAL & \underline{68.0} & \textbf{77.2} & \textbf{69.7} & \textbf{76.2} & \textbf{72.8} & \textbf{74.4}\\
% OREAL Mean & 67.9 & 73.6 & \underline{66.2} & 74.8 & \underline{70.6} & 71.5\\
% OREAL Prob x Ent & 66.5 & 75.2 & 62.1 & 75.8 & 70.0 & 71.0 \\
% OREAL $\delta$ & . & 76.2 & 65.6 & \underline{0.760} & . & \underline{72.6}\\
% OREAL $95\%$ & \textbf{68.5} & \underline{76.6} & . & . & . & . \\
% \hline
% \end{tabular}
% }
% \caption{AuALC of all ablations across all datasets averaged over 10~runs (MONARCH, EndoVis) and 3~runs (Cityscapes, Pascal~VOC) on the ResNet50 backbone. Metrics are computed at the end of the 6~active learning steps. Best scores are in bold, and second best are underlined.}
% \label{tab: ablation}
% \end{table*}

% \section{Experimental Settings}
% We further detail some aspects of our experiments in this section.
% \subsection{Baselines}
% We provide below a detailed explanation of baselines presented in the main paper:
% \begin{description}
%     \item[\RSamp] selects $Q$~random superpixels from~$\U_t$ at each iteration.
%     \item[\BvSBSamp~\cite{BvSB}] estimates the uncertainty of a pixel using the ratio between the most confident and second most confident class posterior. The uncertainty of a superpixel is the average of the pixel uncertainty within it. It then selects the superpixels with the highest uncertainty.
%     \item[\RevisitingSPSamp~\cite{revisiting}] uses the \BvSBSamp~ uncertainty~\cite{BvSB} weighted by the posterior of the class distributions to promote class balancing. Class distributions are computed for each class as the proportion of superpixels predicted to be that class. Their strategy selects the superpixels with the highest weighted uncertainty.
%     \item[\PixelBalSamp~\cite{multi_label_AL}] extends the~\RevisitingSPSamp{} method computing the class distribution for class~$c$ as the sum of the predicted probabilities over all pixels for that class divided by the total number of pixels. The superpixel score is computed as the average of the pixel-wise weighted uncertainties. The weighting requires a hyperparameter~$\nu$, which is set to $\nu=6$ for Cityscapes and $\nu=12$ for Pascal VOC, following the authors' original values. For EndoVis and MONARCH we set~$\nu=12$. As above, their strategy selects superpixels with the highest weighted uncertainty.
%     \item[\CBALSamp~\cite{CBAL}] scores the uncertainty of a sample by calculating a residual entropy obtained from the standard entropy by subtracting the $L^1$-norm between the predicted probability vector and the class counts vector~$\bm{\delta}$.
%     %as defined in Sec.~\ref{sec: annotation_strat}. 
%     The $L^1$-norm is scaled by a factor~$\lambda$, which we set to $\lambda=2$ for all datasets. To adapt the original work from classification to segmentation, we average the pixel-wise entropies and probability vectors over all pixels within each superpixel before computing the residual entropy scores at the superpixel level. The strategy selects the superpixels with the highest residual entropy.
% \end{description}

% \subsection{Data Augmentations}
% We apply data augmentation for training our segmentation model. For MONARCH \cite{COWAL} and EndoVis \cite{endovis}, we use the same data augmentations as in~\cite{COWAL}: MONARCH and EndoVis images are first resized to~$220\times220$ and~$224\times224$, respectively. We then take crops with random scale factors in the range~$(0.85, 1)$ and with random aspect ratios in the range~$\left(\frac{3}{4}, \frac{4}{3}\right)$. All crops are re-scaled back to the initial size of $220\times220$ or~$224\times224$, followed by a random horizontal flipping with a probability of~$0.5$.

% For Cityscapes \cite{cityscapes} and Pascal VOC \cite{pascalVOC}, we start by resizing the images to~$769\times769$ and~$513\times513$ respectively, as done in~\cite{revisiting}. Next, we upscale the images by adding a random number of $\ell$~pixels in both the horizontal and vertical dimensions. The value of $\ell$~follows a uniform distribution~$\mathcal{U}(0, 300)$ for Cityscapes and $\mathcal{U}(0, 200)$ for Pascal VOC. After upscaling, we center-crop the images to their original size of~$769\times769$ or~$513\times513$ and randomly flip them horizontally with a probability of~$0.5$.

% \subsection{Running Time}
% The time needed to run our AL pipeline for one seed is respectively 24, 8, 5, and 6 hours for Cityscapes, Pascal VOC, MONARCH, and EndoVis. This time corresponds to a complete AL pipeline, from iterations 0 to 5, per seed. The time needed to complete the AL pipeline is roughly the same for all AL methods. We used a single RTX3090Ti (24GB) for our experiments.

% \subsection{Reproducibility}
% For all AL methods, the initial training phase, denoted as round 0, utilizes the same training dataset to train the segmentation model. An identical test score is observed across different methods at the conclusion of round 0. Although setting the seed for random number generators in numpy and pytorch contributed to reproducibility, it proved insufficient for ensuring perfect consistency. A crucial modification was made to the segmentation model, specifically to the interpolation layer within DeepLabV3 \cite{deeplabV3}. By altering the interpolation mode from bilinear to nearest, we achieved deterministic computation, ensuring that the model behavior became predictable and reproducible. Since different AL methods when trained on the same dataset at round 0 achieve the same test score, in the following AL iterations (1 to 5), the difference observed between AL methods is only attributable to the labeled set each of them built.

% \subsection{Weak Labeling of Patches}
% \OurSamp~was designed under the assumption that superpixels only require one click to be annotated. Given a budget of $Q$ clicks, we can thus annotate $Q$ superpixels. However, when patches are weakly labeled \cite{multi_label_AL}, the annotator declares all the classes present in the superpixel and requires one click per class. Thus, some superpixels, with more than one class, would require more than one click to be annotated. With a budget $Q$, we will then have less than $Q$ annotated superpixels.

% In the case of \OurSamp, once the list of superpixel numbers to be selected per class $\delta$ (the numbers in $\delta$ sum up to $Q$) is computed, starting with the first class, we select all the required number of superpixels for this class before proceeding for the next class. When superpixels only require one click to be annotated, we are sure to select the required number of superpixels for all classes. However, when superpixels require more than one click, our budget can be exhausted before we can start selecting superpixels for the last classes. To resolve this issue, we simply select one superpixel per class and proceed to the next class. This way we ensure all classes are equally selected. Our selection procedure stops when the annotation budget is exhausted and the rate at which this budget decreases will depend on the number of classes per superpixel we encounter.

% \subsection{Other details}
% \textbf{AL initialization.} After validation split, the set of labeled frames~$\A_1$ is initialized with $Q$~random superpixels throughout the training set. The remaining superpixels are assigned to the complementary set of unlabeled frames~$\U_1$. 

% \textbf{Background class.} We applied the special treatment for background classes of Sec.~\ref{sec:background_class} to the MONARCH, EndoVis, and Pascal~VOC datasets. This treatment was omitted for the \emph{void} class of Cityscapes because it is not used to train or evaluate the model.

% \section{Additional Results}
% We show in this section complementary results that did not fit in the main paper due to lack of space.

% \subsection{Active Learning Curves}
% Fig.~\ref{fig: AL_results RN101} shows the Active Learning curves using the ResNet101 backbone and Fig.~\ref{fig: AL_results ViT} shows the Active Learning curves using the ViT backbone.

% \begin{figure*}[t]
%     \includegraphics[width=0.5\linewidth]{figures/cityscapes_ResNet101.pdf}
%     \includegraphics[width=0.5\linewidth]{figures/pascal_VOC_ResNet101.pdf}
%     \medskip
%     \includegraphics[width=0.5\linewidth]{figures/auris_ResNet101.pdf}
%     \includegraphics[width=0.5\linewidth]{figures/intuitive_ResNet101.pdf}
%    \caption{Comparison of different sampling strategies.
%    Values are averaged over 3 training-validation splits for Cityscapes \cite{cityscapes}, Pascal VOC \cite{pascalVOC}, and 10 training-validation splits for EndoVis \cite{endovis}, MONARCH \cite{COWAL} on the ResNet101 backbone. Error bars indicate one standard deviation.}
% \label{fig: AL_results RN101}
% \end{figure*}

% \begin{figure*}[t]
%     \includegraphics[width=0.5\linewidth]{figures/cityscapes_ViT.pdf}
%     \includegraphics[width=0.5\linewidth]{figures/pascal_VOC_ViT.pdf}
%     \medskip
%     \includegraphics[width=0.5\linewidth]{figures/auris_ViT.pdf}
%     \includegraphics[width=0.5\linewidth]{figures/intuitive_ViT.pdf}
%    \caption{Comparison of different sampling strategies.
%    Values are averaged over 3 training-validation splits for Cityscapes \cite{cityscapes}, Pascal VOC \cite{pascalVOC}, and 10 training-validation splits for EndoVis \cite{endovis}, MONARCH \cite{COWAL} on the ViT backbone. Error bars indicate one standard deviation.}
% \label{fig: AL_results ViT}
% \end{figure*}

% \subsection{mIoU improvement using max aggregation}
% Tab.~\ref{tab: mIoU tab results} shows the average mIoU improvement across all AL iterations from using \MeanAgg~to \MaxAgg. On average, all AL methods benefit from using \MaxAgg~instead of \MeanAgg~with the Pascal VOC that has an average mIoU improvement of 1.54 across all AL methods and backbones.

% \begin{table*}[h!]
% \centering
% \begin{tabular}{l|c|c|c|c|c|c}
% \hline
% \textbf{Method} & \diagbox[width=8em]{\textbf{Backbone}}{\textbf{Datasets}} & \multicolumn{1}{c|}{\textbf{MONARCH}} & \multicolumn{1}{c|}{\textbf{PASCAL VOC}} & \multicolumn{1}{c|}{\textbf{ENDOVIS}} & \multicolumn{1}{c|}{\textbf{CITYSCAPES}} & \textbf{Average} \\
% \hline
% \hline
% BvSB & RN50 & \textcolor{green}{1.47} & \textcolor{green}{1.36} & \textcolor{green}{0.29} & \textcolor{red}{-0.19} & \textcolor{green}{0.73} \\
% revisiting SP & RN50 & \textcolor{green}{1.67} & \textcolor{green}{0.32} & \textcolor{red}{-0.18} & \textcolor{green}{0.41} & \textcolor{green}{0.56} \\
% Pixel Bal & RN50 & \textcolor{red}{-1.31} & \textcolor{green}{1.54} & \textcolor{green}{0.39} & \textcolor{red}{-0.41} & \textcolor{green}{0.05} \\
% CBAL & RN50 & \textcolor{red}{-0.31} & \textcolor{red}{-0.10} & \textcolor{red}{-0.14} & \textcolor{green}{0.07} & \textcolor{red}{-0.12} \\
% OREAL (ours) & RN50 & \textcolor{green}{1.25} & \textcolor{green}{2.18} & \textcolor{green}{0.65} & \textcolor{green}{0.18} & \textcolor{green}{1.07} \\
% \hline
% BvSB & RN101 & \textcolor{green}{0.48} & \textcolor{green}{1.93} & \textcolor{green}{0.62} & \textcolor{green}{0.35} & \textcolor{green}{0.85} \\
% revisiting SP & RN101 & \textcolor{red}{-0.70} & \textcolor{green}{1.04} & \textcolor{green}{0.05} & \textcolor{green}{1.32} & \textcolor{green}{0.43} \\
% Pixel Bal & RN101 & \textcolor{red}{-0.10} & \textcolor{green}{1.93} & \textcolor{green}{0.89} & \textcolor{green}{1.64} & \textcolor{green}{1.09} \\
% CBAL & RN101 & \textcolor{red}{-0.83} & \textcolor{red}{-0.81} & \textcolor{red}{-0.16} & \textcolor{green}{0.34} & \textcolor{red}{-0.36} \\
% OREAL (ours) & RN101 & \textcolor{red}{-0.40} & \textcolor{green}{1.82} & \textcolor{green}{0.40} & \textcolor{red}{-0.06} & \textcolor{green}{0.44} \\
% \hline
% BvSB & ViT & \textcolor{green}{2.27} & \textcolor{green}{3.32} & \textcolor{green}{0.70} & \textcolor{red}{-0.30} & \textcolor{green}{1.50} \\
% revisiting SP & ViT & \textcolor{green}{1.66} & \textcolor{green}{3.20} & \textcolor{green}{0.17} & \textcolor{red}{-0.10} & \textcolor{green}{1.23} \\
% Pixel Bal & ViT & \textcolor{green}{1.95} & \textcolor{green}{3.24} & \textcolor{green}{0.71} & \textcolor{green}{0.03} & \textcolor{green}{1.48} \\
% CBAL & ViT & \textcolor{red}{-0.84} & \textcolor{green}{0.75} & \textcolor{green}{0.10} & \textcolor{red}{-0.46} & \textcolor{red}{-0.11} \\
% OREAL (ours) & ViT & \textcolor{red}{-0.64} & \textcolor{green}{2.47} & \textcolor{green}{0.24} & \textcolor{green}{0.66} & \textcolor{green}{0.68} \\
% \hline
% \hline
% \textbf{Average} & & \textcolor{green}{0.37} & \textcolor{green}{1.54} & \textcolor{green}{0.33} & \textcolor{green}{0.30} & \textcolor{green}{0.64} \\
% \hline
% \end{tabular}
% \caption{Average mIoU improvement from using \MeanAgg~to \MaxAgg~across all AL iterations of all strategies across all datasets. A positive number $n$ means, \MaxAgg~has achieved a higher mIoU than \MeanAgg~by a margin of $n$.}
% \label{tab: mIoU tab results}
% \end{table*}

% \subsection{Selected superpixels on additional datasets}
% The main paper showed selected superpixels for the Pascal VOC and EndoVis datasets. Fig.~\ref{fig:sampled patches 2} shows additional superpixels selected for the Cityscapes and MONARCH datasets. Similar to the selected superpixels on the Pascal VOC and EndoVis datasets, \MaxAgg~has selected more regions at the boundaries between objects.

% \begin{figure*}[t]
%     \includegraphics[width=\linewidth]{figures/cityscapes_selected_patches.pdf}
%     \includegraphics[width=\linewidth]{figures/intuitive_selected_patches.pdf}
%     \includegraphics[width=\linewidth]{figures/auris_selected_patches.pdf}
%    \caption{Selected superpixel regions of different sampling strategies. On average, we observe that when using the max aggregation, all sampling methods tend to select more regions around the boundary of objects.}
% \label{fig:sampled patches 2}
% \end{figure*}

% \subsection{Superpixel annotated frames}
% Fig.~\ref{fig: SP annotated frames} shows examples of superpixel annotated frames using the dominant labeling scheme. For datasets like Pascal VOC, Endovis, and MONARCH the qualitative quality of the superpixel annotated labels is correct when compared to the original segmentation masks. This explains the small performance gap between using the original segmentation masks and the superpixel annotated masks in Tab. 2 of the main paper. In the case of Cityscapes which display much more complex sceneries, the use of superpixel annotation had a bigger impact on decreasing the segmentation mask quality. As such, the performance gap in Tab. 2 of the main paper for Cityscapes becomes bigger.

% \begin{figure*}[t]
%     \includegraphics[width=\linewidth]{figures/DOvsPR_pascal_VOC.pdf} 
%     \includegraphics[width=\linewidth]{figures/DOvsPR_intuitive.pdf}
%     \includegraphics[width=\linewidth]{figures/DOvsPR_cityscapes.pdf}
%     \includegraphics[width=\linewidth]{figures/DOvsPR_auris.pdf}
%    \caption{For each pair of images, the original segmentation mask is on the left and the segmentation mask annotated using superpixel dominant labeling is on the right. Each row shows respectively pair of images from the Pascal VOC, EndoVis, Cityscapes, MONARCH datasets. \RebuttalText{The complete mIoU of the dominant labels are 93.7, 83.3, 74.6, and 82.3, for Pascal VOC, EndoVis, Cityscapes, and MONARCH respectively.}}
% \label{fig: SP annotated frames}
% \end{figure*}

% \subsection{Weak Labeling of Patches}
% Fig.~\ref{fig: AL_results MUL} shows the AL curves for the results presented in Tab.~4 of the main paper. Finally, Tab.~\ref{tab: MUL resutls} shows the average mIoU improvement across all AL iterations from using \MeanAgg~to \MaxAgg~in the case of the weak labeling scheme. While the performance gap is marginal on Pascal VOC, it is significant on Cityscapes which benefits from \MaxAgg.

% \RebuttalText{\subsection{Gini Index}
% To assess how well each AL method balances the different classes of a dataset, we calculate the Gini Index~\cite{gini} for datasets built by each AL method at the end of the AL iterations and show the results in Tab.~\ref{tab: gini_index}. The Gini index is
% equal to 0 for a list of uniform values and converges to 1
% otherwise. Overall we can see that~\OurSamp~built a better class-balanced dataset than the other AL methods. In the case of \OurSamp, using mean aggregation should be more precise at balancing the dataset than using max aggregation. This is the case for datasets such as Cityscapes and EndoVis but not for MONARCH and Pascal VOC. We think this behavior is caused by the fact that images from MONARCH and Pascal VOC display on average less than 2 classes per image against 6 to 12 classes for EndoVis and Cityscapes. Since the task of balancing classes is more difficult when having multiple classes per image, the difference between a better and worse balancing metric is more noticeable.}

% \RebuttalText{\subsection{AuALC improvement per class}
% Fig.~\ref{fig: AuALC improvement City} and \ref{fig: AuALC improvement VOC} display the AuALC improvement per class of \OurSamp~against all baselines for the Cityscapes and Pascal VOC dataset respectively. Overall, \OurSamp~could achieve better results than baseline on tail classes, whether AL methods are using the mean or max aggregation.}

% \RebuttalText{\subsection{Entropy Map}
% Fig.~\ref{fig: entropy map} shows examples of entropy maps for Pascal VOC images. For the majority of superpixels located at the border of objects, we observe that only a few pixels in the proximity of the object boundary have high entropy. Hence using max aggregation for those superpixels greatly differs from using mean aggregation and allows the uncertainty-based AL methods to select such superpixels.}

% \begin{figure*}[t]
%     \includegraphics[width=0.5\linewidth]{figures/cityscapes_ResNet50 - Stage 1_MUL.pdf}
%     \includegraphics[width=0.5\linewidth]{figures/cityscapes_ResNet50 - Stage 2_MUL.pdf}
%     \medskip
%     \includegraphics[width=0.5\linewidth]{figures/pascal_VOC_ResNet50 - Stage 1_MUL.pdf}
%     \includegraphics[width=0.5\linewidth]{figures/pascal_VOC_ResNet50 - Stage 2_MUL.pdf}
%    \caption{Comparison of different sampling strategies when patches are weakly annotated following the method proposed by \cite{multi_label_AL}.
%    Values are averaged over 3 training-validation splits. Error bars indicate one standard deviation.}
% \label{fig: AL_results MUL}
% \end{figure*}

% \begin{table}[h!]
% \centering
% \begin{tabular}{l|c|c|c}
% Method & Stage & \multicolumn{1}{c|}{Pascal VOC} & \multicolumn{1}{c}{Cityscapes} \\ 
%  & & mean - max & mean - max \\
% \hline
% \hline
% BvSB & 1 & \textcolor{red}{-0.13} & \textcolor{green}{0.40} \\
% revisiting SP & 1 & \textcolor{green}{0.41} & \textcolor{green}{0.98} \\
% Pixel Bal & 1 & \textcolor{red}{-0.15} & \textcolor{green}{0.24} \\
% OREAL & 1 & \textcolor{red}{-0.17} & \textcolor{green}{0.26} \\
% \hline
% BvSB & 2 & \textcolor{red}{-0.11} & \textcolor{green}{0.42} \\
% revisiting SP & 2 & \textcolor{red}{-0.14} & \textcolor{green}{1.33} \\
% Pixel Bal & 2 & \textcolor{red}{-0.34} & \textcolor{green}{0.42} \\
% OREAL & 2 & \textcolor{green}{0.07} & \textcolor{green}{0.16} \\
% \hline
% \hline
% \textbf{Average} & & \textcolor{red}{-0.07} & \textcolor{green}{0.65} \\
% \hline
% \end{tabular}
% \caption{Average mIoU improvement from using \MeanAgg~to \MaxAgg~across all AL iterations of all strategies across all datasets when patches are annotated using the weak labeling scheme \cite{multi_label_AL}. A positive number $n$ means, \MaxAgg~has achieved a higher mIoU than \MeanAgg~by a margin of $n$.}
% \label{tab: MUL resutls}
% \end{table}

% \begin{table}[t]
% \centering
% \resizebox{0.96\columnwidth}{!}{
% \begin{tabular}{c | c | c | c | c}
%     Methods & \multicolumn{1}{c|}{MONARCH} & \multicolumn{1}{c}{PASCAL VOC} & \multicolumn{1}{c}{CITYSCAPES} & \multicolumn{1}{c}{ENDOVIS} \\
%     & mean - max & mean - max & mean - max & mean - max \\
%     \hline
%     Random & 0.42 & 0.67 & 0.25 & 0.41 \\
%     BvSB & 0.35 - \textbf{0.40} & 0.61 - \textbf{0.63} & \textbf{0.35} - \textbf{0.35} & 0.45 - \textbf{0.46} \\
%     Revisiting SP & 0.40 - \textbf{0.47} & 0.63 - \textbf{0.66} & 0.42 - \underline{\textbf{0.56}} & 0.49 - \textbf{0.52} \\
%     Pixel Bal & 0.42 - \textbf{0.53} & 0.60 - \textbf{0.72} & \textbf{0.39} - 0.38 & 0.50 - \textbf{0.52} \\
%     CBAL & \underline{0.56} - \underline{\textbf{0.59}} & 0.65 - \textbf{0.66} & \textbf{0.48} - 0.47 & \textbf{0.55} - \textbf{0.55} \\
%     OREAL (ours) & \underline{0.56} - \underline{\textbf{0.59}} & \underline{0.83} - \underline{\textbf{0.86}} & \underline{\textbf{0.54}} - 0.51 & \underline{\textbf{0.57}} - \underline{0.56} \\
%     \hline
% \end{tabular}
% }
% \caption{\RebuttalText{"1 - Gini Index" of class distribution of datasets built by different AL methods at the end of AL iterations on the ResNet50 model. The best value between each pair of mean - max aggregation is in bold and the best methods for each column of mean - max aggregation is underlined.}}
% \label{tab: gini_index}
% \end{table}

% \begin{figure*}[t]
%     \includegraphics[width=0.5\linewidth]{figures/cityscapes_tailClass_dist.pdf} 
%     \includegraphics[width=0.5\linewidth]{figures/cityscapes_tailClass_dist.pdf} 
%     \\
%     \includegraphics[width=0.5\linewidth]{figures/cityscapes_tailClass_score.pdf}
%     \includegraphics[width=0.5\linewidth]{figures/cityscapes_tailClass_RN50_score_max.pdf}
%    \caption{\RebuttalText{Top 2 graphs show the distribution of Cityscapes classes. The bottom 2 graphs show the relative AuALC improvement of OREAL vs. baselines for each Cityscapes class (positive indicates OREAL is better). The bottom left graph is for methods using the mean aggregation and the bottom right is for methods using the max aggregation.}}
% \label{fig: AuALC improvement City}
% \end{figure*}

% \begin{figure*}[t]
%     \includegraphics[width=0.5\linewidth]{figures/pascal_VOC_tailClass_dist.pdf} 
%     \includegraphics[width=0.5\linewidth]{figures/pascal_VOC_tailClass_dist.pdf} 
%     \\
%     \includegraphics[width=0.5\linewidth]{figures/pascal_VOC_tailClass_score.pdf}
%     \includegraphics[width=0.5\linewidth]{figures/pascal_VOC_tailClass_RN50_score_max.pdf}
%    \caption{\RebuttalText{Top 2 graphs show the distribution of Pascal VOC classes. The bottom 2 graphs show relative AuALC improvement of OREAL vs. baselines for each Pascal VOC class (positive indicates OREAL is better). The bottom left graph is for methods using the mean aggregation and the bottom right is for methods using the max aggregation.}}
% \label{fig: AuALC improvement VOC}
% \end{figure*}

% \begin{figure*}[h]
%     \includegraphics[width=0.33\linewidth]{figures/entropy_map_1.pdf} 
%     \includegraphics[width=0.33\linewidth]{figures/entropy_map_2.pdf}
%     \includegraphics[width=0.33\linewidth]{figures/entropy_map_3.pdf}
%    \caption{\RebuttalText{Entropy map of 3 images from Pascal VOC. The images are split into superpixels. Pixel with high entropy belongs respectively to the Dog, Bird, and Cow classes. On the border of these classes, some pixels overflow and belong to superpixels surrounding the classes. Hence using max aggregation for those border superpixels will emphasize the few pixels that have high entropy located at the border with the classes.}}
% \label{fig: entropy map}
% \end{figure*}

% {\small
% \bibliographystyle{ieee_fullname}
% \bibliography{main}
% }

% \end{document}
